# Supplementary material for: Unmasking charge transfer in the Misfits: ARPES and ab initio prediction of electronic structure in layered incommensurate systems without artificial strain
Source: arXiv:2407.05465 source file (2024-07-07)
Supplement: Supplementary file 1 [file Supplemental_Materials.pdf]

# Supplemental Materials

July 2024

## S1 DFT methodology

All *ab initio* calculations in this work employ our group's JDFTx software package [34] using GBRV ultrasoft pseudopotentials [35] and the generalized gradient approximation (GGA) [36] to the exchange-correlation functional, and employ a plane-wave basis with a 20 hartree cutoff throughout the crystal and 100 hartree cutoff for the atomic core charge corrections. Our Brillouin-zone integrals use a thermal Fermi distribution for the electrons of 0.001 Hartree (approximately room temperature) to replicate experimental conditions and Monkhorst-Pack sampling of  $n_{kx} \times 6 \times 3$ , where  $n_{kx} = 4, 3, 3, 2, 2$  for the  $n_{\text{La}} = 4, 6, 8, 10, 12$  supercells, respectively. Finally, we relaxed all ionic and lattice degrees of freedom to within an energy tolerance of  $10^{-2}$  meV/atom.

## S2 Interlayer charge transfer methodology

As described in the main text, and elaborated here for the interested reader, we compute the interlayer charge transfer by first determining the ground-state electron density for the MINT proxy system in question,  $n_{\text{misfit}}(r)$  (e.g.,  $(\text{LaSe})_{10}(\text{NbSe}_2)_{24}$ ). We then freeze the atomic coordinates and extract the LaSe strip from the relaxed MINT proxy system and compute the ground-state electron density of this isolated component,  $n_{\text{LaSe}}(r)$ , while keeping the ionic positions and the lattice fixed. We then follow the exact same procedure to perform a calculation for the  $\text{NbSe}_2$  substrate in isolation to obtain its ground-state electron density,  $n_{\text{NbSe}_2}(r)$ . These real-space electron densities are easily obtained as standard JDFTx outputs.

Next, we subtract the isolated electron densities from that of the MINT-proxy misfit system:

$$\Delta n(r) = n_{\text{misfit}}(r) - n_{\text{LaSe}}(r) - n_{\text{NbSe}_2}(r). \quad (\text{S1})$$

This represents the change in electron density when the LaSe strip and  $\text{NbSe}_2$  substrate are allowed to interact electronically. To obtain the net interlayer charge transfer from  $\Delta n(r)$ , we then simply integrate over the spatial volume associate with the  $\text{NbSe}_2$  substrate. Although the boundary between the LaSe and  $\text{NbSe}_2$  layers has no unique definition, we define it in a consistent and physically motivated manner as follows.

First, we integrate all relevant charge-densities in planes orthogonal to the z-axis (interlayer stacking direction) to obtain one dimensional functions:

$$\Delta n(z) = \int \Delta n(r) dx dy, \quad n_a(z) = \int n_a(z) dx dy, \text{ where } a = \text{misfit, LaSe, NbSe}_2. \quad (\text{S2})$$

We then define the boundaries between the LaSe and  $\text{NbSe}_2$  layers to be the points  $z = z_c$  between the two layers defined so that  $n_{\text{misfit}}(z_c)$  is at a minimum. Since  $(\text{LaSe})_{1.14}(\text{NbSe}_2)_2$  is periodically stacked and not just a single interface (as in the original MINT approach), we actually find two values of  $z_c$ , one below the LaSe layer,  $z_{c1}$ , and one above,  $z_{c2}$ . We then define our final interlayer charge transfer for this MINT proxy system as

$$\Delta Q = \int_{z_{c1}}^{z_{c2}} \Delta n(z) dz. \quad (\text{S3})$$

Because  $\Delta n(z)$  is a discrete array, in practice we round  $z_{c1}$  and  $z_{c2}$  to the nearest integer indexes on the spatial grid for the charge density. The reported errors on  $\Delta Q$  in Figure 1 of the main text correspond to the change in  $\Delta Q$  upon a discrete change in  $z_{c1}$  and  $z_{c2}$  by one unit in either direction.

The interlayer charge transfer of bulk incommensurate  $(\text{LaSe})_{1.14}(\text{NbSe}_2)_2$  can then be extracted from the limiting value of  $\Delta Q$  across the MINT proxy sequence, Figure 1(b) in the main text. For each LaSe strip size in our MINT sequence  $n_{\text{La}} = 4, 6, 8, 10, 12$ , we compute  $\Delta Q$  as described above from the fully relaxed atomic positions, and then repeat the calculation for  $\Delta Q$  across multiple relative shifts of the LaSe strip from its fully relaxed position. Each data point in Figure 1(b) is the average of  $\Delta Q$  over these multiple shifts with new relaxations, and the reported error bars are the average over the errors on  $\Delta Q$  for each shift, assuming independence. The error reported for the final extrapolated incommensurate charge transfer is determined from the linear fit using standard propagation of errors with the individual errors on each data point determined as above.

### S3 ARPES methodology

All single crystal samples were cleaved in ultra high vacuum (UHV) to prepare pristine surfaces. ARPES measurements were taken with a Scienta Omicron DA30 electron analyzer equipped with a Fermion Instruments BL1200s discharge lamp using monochromated He-I photons at 21.2 eV. The samples were held at 7 K during measurements, and the analyzer was set to a nominal energy resolution of 9 meV.

### S4 Real space weighting procedure

Because every MINT proxy system contains both an isolated flake/strip of one material over a periodic substrate of another, there will always be a region that contains only the substrate and the vacuum gap between periodic images of the flake/strip. However, only the “covered” region, containing both materials, is representative of the bulk incommensurate system. While these gap regions do not significantly impact our procedure for extracting charge transfers and are well accounted by our finite size scaling extrapolation, these regions do impact significantly the convergence of the momentum-resolved density of states (MRDOS)  $n(q, \epsilon)$  that we use to predict ARPES measurements in the main text.

To account for the gaps in the context of ARPES, we introduce an additional weighting factor at each band and kpoint,  $p_{nk}$ , in our expression for the MRDOS,

$$n(q, \epsilon) = \sum_n \int_{BZ} dk p_{nk} |\psi_{nk}(q)|^2 \delta(\epsilon - \epsilon_n(k)), \quad (\text{S4})$$

where the weight  $p_{nk}$  represents the probability of finding the electrons in the eigenstate  $\psi_{nk}$  of the MINT proxy system to be in the “covered” (*e.g.*, non-gap) region  $V_{\text{cov}}$ . Expressed in terms of Wannier functions, these weights are

$$p_{nk} = \int_{V_{\text{cov}}} |\psi_{nk}(r)|^2 dr = \int_{V_{\text{cov}}} \left| \frac{1}{\sqrt{N}} \sum_R \sum_m U_{nm}(k) w_{mR}(r) e^{ikR} \right|^2 dr. \quad (\text{S5})$$

Here,  $w_{mR}(r)$  is the  $m^{\text{th}}$  real space Wannier function centered in the unit cell indexed by  $R$ , where  $R$  indexes the  $N$  unit cells in the macroscopic crystal. ( $N$  will eventually cancel in the final expression.)

Because direct use of (S5) is very inefficient for practical calculations because floating point operations on  $\psi_{nk}(r)$  or  $w_{mR}(r)$  are very expensive and are to be performed at every kpoint  $k$ , we reduce the computational scaling by expressing  $p_{nk}$  in terms of overlap integrals between Wannier functions that can be pre-computed independent of the desired k-points,

$$\begin{aligned} p_{nk} &= \int_{V_{\text{cov}}} \left( \frac{1}{\sqrt{N}} \sum_{R'} \sum_{m'} U_{nm'}^*(k) w_{m'R'}(r) e^{-ikR'} \right) \frac{1}{\sqrt{N}} \sum_R \sum_m U_{nm}(k) w_{mR}(r) e^{ikR} dr \\ &= \int_{V_{\text{cov}}} \frac{1}{N} \sum_{R, R'} \sum_{m, m'} U_{nm'}^*(k) U_{nm}(k) w_{m'R'}(r) w_{mR}(r) e^{ik(R-R')} dr \\ &= \frac{1}{N} \sum_{R, R'} e^{ik(R-R')} \sum_{m, m'} U_{nm'}^*(k) U_{nm}(k) \int_{V_{\text{cov}}} w_{m'R'}(r) w_{mR}(r) dr. \end{aligned} \quad (\text{S6})$$

(Note that the ordinarily expected orthonormality among the Wannier functions does not apply here because the integration is restricted to the “covered” region and is not over all of space.) Next, by letting  $R' = R + \Delta R$ , and

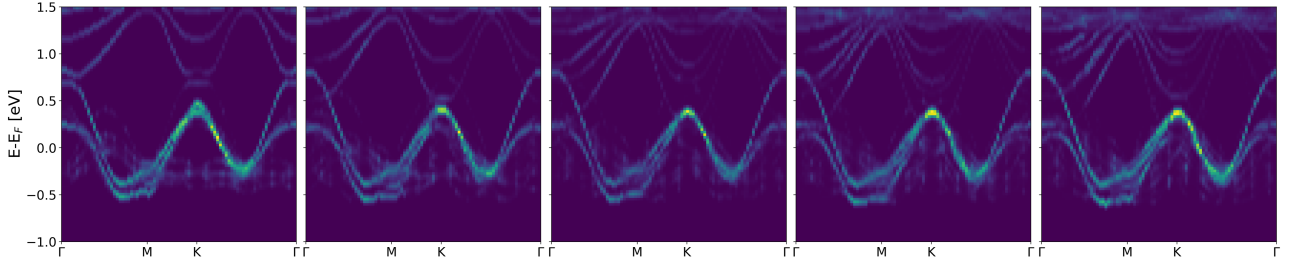

Figure S1: Momentum resolved density of states (MRDOS) of the bulk  $(\text{LaSe})_{1.14}(\text{NbSe}_2)_2$  proxy sequence for  $n_{\text{La}}=4,6,8,10,12$ . Convergence is reached by the end of the subsequence shown.

utilizing the discrete translational symmetry of Wannier functions between unit cells the expression further reduces to

$$\begin{aligned}
 p_{nk} &= \frac{1}{N} \sum_{R, \Delta R} e^{-ik\Delta R} \sum_{m, m'} U_{nm'}^*(k) U_{nm}(k) \int_{V_{\text{cov}}} w_{m'R+\Delta R}(r) \cdot w_{mR}(r) dr \\
 &= \sum_{\Delta R} e^{-ik\Delta R} \sum_{m, m'} U_{nm'}^*(k) U_{nm}(k) \int_{V_{\text{cov}}} w_{m'\Delta R}(r) \cdot w_{m0}(r) dr
 \end{aligned} \tag{S7}$$

Now, the overlap integrals involving the real-space Wannier functions need only be computed for each pair of Wannier functions  $(m0, m'\Delta R)$ , where  $w_{m0}(r)$  lies in the central unit cell and  $w_{m'\Delta R}(r)$  lies in the unit cell translated by  $\Delta R$  from the central unit cell. In practice the sum over  $\Delta R$  can be truncated to include only the closest neighboring unit cells (or slightly larger region as appropriate) if the Wannier functions are sufficiently localized.

## S5 MINT ARPES convergence sequence

Figure S1 shows the sequence convergence of the MINT-Sandwich predicted momentum resolved density of states (MRDOS) for the bulk misfit material. Note that, even at  $n_{\text{La}} = 4$ , we are able to predict the MRDOS reasonably well. We do find important, somewhat subtle changes that do converge by the  $n_{\text{La}} = 12$  member of the sequence. Specifically, the top of the lower energy Fermi level crossing band at  $\Gamma$  point the breaks off at  $n_{\text{La}} = 10, 12$ , indicating a localization of those particular states.

## S6 MINT band-doping extrapolation

The effective doping of the  $\text{NbSe}_2$  layers corresponds to the number of electrons that fill the Fermi-level crossing  $\text{NbSe}_2$  bands in order to effect the rigid band shift (as compared to bulk  $\text{NbSe}_2$ ) observed in both our *ab initio* calculations and ARPES data. We again emphasize that this effective doping is not equivalent to the interlayer charge transfer. The effective doping for each member of the MINT-Sandwich prototype sequence can, however, be calculated in much the same way as the net interlayer charge transfer, and its value in the infinite incommensurate system can be extracted from an analogous fit. To compute the effective doping of each member of the MINT-Sandwich sequence, we utilize the energy gap that we find between the lower valence bands and the Fermi-level crossing bands in all three cases (isolated  $\text{LaSe}$ , isolated  $\text{NbSe}_2$ , and their MINT combination). To determine the doping into the Fermi-level  $d$ -bands, we then subtract the electron densities of the valence bands below this gap (which represent all electrons in non-Fermi-level crossing bands) from the total electron densities to extract the electron densities of the Fermi-level crossing bands in all three systems. Then, following the same procedure as we did for the total electron density, subtract the sum of the electron densities (in the Fermi-level crossing bands) of the isolated  $\text{LaSe}$  and  $\text{NbSe}_2$  systems from that of their interacting misfit combination and integrate over the extent of the  $\text{NbSe}_2$  to obtain the effective doping of the  $\text{NbSe}_2$  layers. Figure S2 plots this effective doping across the MINT-Sandwich prototype sequence. The value of the doping converges to its limiting value of  $0.921 \text{ e}^-/\text{La} = 0.525 \text{ e}^-/\text{Nb}$  as reported in the main text. It is extracted by performing a linear fit to the data points computed from the four largest MINT proxy systems, as described above for the total electron density.

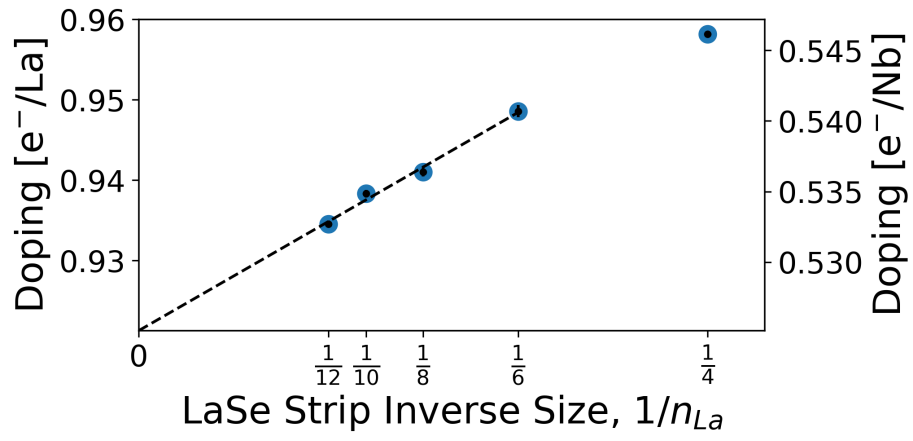

Figure S2: Effective doping of the NbSe<sub>2</sub> layer versus inverse strip size for the MINT-Sandwich prototype sequence, with best fit linear relationship (dashed line).
